# Supplementary material for: Connectivity dynamics in the vitrification of colloidal liquids
Source: arXiv:1612.00704 ancillary file (2016-12-02)
Supplement: Supplementary file 1 [file SuppInfo_Higler_etal.pdf]

# Supplemental Information for:
# *Connectivity dynamics in the vitrification of colloidal liquids*

Ruben Higler,[1] Johannes Krausser,[2] Jasper van der Gucht,[1] Alessio Zaccone,[2] and Joris Sprakel[1,*]

[1] *Physical Chemistry and Soft Matter, Wageningen University and Research, Wageningen, 6708 WE, The Netherlands*

[2] *Department of Chemical Engineering and Biotechnology, and Cavendish Laboratory, University of Cambridge, Cambridge, CB2 3RA, UK*

(Dated: December 2, 2016)

* joris.sprakel@wur.nl

# I. SYNTHESIS

All materials are purchased from Sigma-Aldrich (SA) and used as received, unless specified otherwise. For the synthesis of polymethyl methacrylate (PMMA) colloidal particles we use: Methyl methacrylate (MMA, SA M55909), Methacrylic acid (MA, SA 155721), Hexane (SA 208752), Mineral Oil BioUltra (SA 69794), 2,2'-Azobis(2-methylpropionitrile) (AIBN, SA 441090), 1-Octanethiol(SA 471836), and 3,3'-Dioctadecyloxacarbocyanine Perchlorate (DiO, ThermoFischer Scientific D-275). For the synthesis of Poly(12-hydroxystearic acid)-graft-poly(methyl methacrylate) (PHSA-g-PMMA) we use: 12-Hydroxystearic Acid (TCI Chemicals, H0308), Toluene (SA, 179965), Methanesulfonic Acid (SA 471356), 4-*tert*-Butylcatechol (SA 124249), Glycidyl methacrylate (GMA, SA 151238), N,N-Dimethyldodecylamine (SA 284386), Ethyl acetate (SA 16371), and Butyl acetate (SA 537454). We also use *cis*-Decahydronaphthalene (cDec, TCI Chemicals D0009), Tetrachloroethylene (TCE, SA 270393), and Docusate sodium salt (AOT, SA 86140).

## A. Synthesis of poly(methyl methacrylate)-*graft*-poly(12-hydroxystearic acid)

Our synthetic procedure for poly(methyl methacrylate)-*graft*-poly( 12-hydroxystearic acid) (PMMA-g-PHSA), the stabiliser used in the synthesis of colloidal PMMA particles, follows the general three-step procedure as detailed in literature [1], with some minor changes. *Step I -* We begin by creating oligomers of 12-Hydroxystearic acid (HSA) aiming for oligomers of around 5 monomers in length, using a polycondensation reaction. To this end we weigh 50 g HSA and 9 g toluene in a 500 mL two necked round-bottom flask equipped with a reflux condenser and a 15 mL Dean-Stark trap, with 12 mL of toluene added to receiver leg. We heat the setup via an oil bath set at 110 $^{\circ}C$ and wait for the HSA to fully melt and dissolve in the toluene, while vigorously stirring the solution. After the HSA has fully dissolved we add 0.11 g of methanesulfonic acid and set the temperature of the oil bath to 150 $^{\circ}C$. We let the reaction reflux for 20 hours, during which the reaction goes from a very pale yellow to a dark brown in colour and the viscosity of the solution increases strongly. During the condensation reaction a total of $\sim$1.5 $mL$ of water are extracted from the flask into the Dean-Stark trap. *Step II -* After 20 hours we empty the receiver leg of the Dean-Stark trap and add 20 mL of toluene to the reaction. We azeotropically distill 15 ml of the added toluene to remove all condensation water from the reaction. We then react the terminal carboxylic group on the PHSA with the epoxide of glycidyl methacrylate (GMA), to create reactive PHSA macromonomers. In a separate beaker we combine 5.2 g GMA, 0.073 g *tert*-Butylcatechol, 0.20 g *N,N*-Dimethyldodecylamine, and 10 g toluene. We add this solution to the refluxing reaction and let allow it to react for another 7 hours while stirring vigorously. After this the reaction is cooled en stored at 4°C until further use. *Step III -* In the third step we co-polymerize MMA and the PHSA macromonomer, to create the PMMA-*graft*-PHSA stabiliser. We prepare a mixture of 31 g of the PHSA macromonomer, as synthesised in steps I & II, 9.2 g toluene, 18.32 g methyl metacrylate, 2.05 g glycidyl methacrylate, and 0.307 g AIBN. We slowly add this mixture dropwise, using a syringe pump, over a period of three hours to a round-bottom flask equipped with a reflux condenser, containing 13.94 g ethyl acetate and 6.97 g butyl acetate which is immersed in a 110 $^{\circ}C$ oil bath. After the reaction mixture has been added to the flask we let the reaction proceed under reflux for two hours after which we add a solution of 140 mg AIBN in 1.5 $g$ ethyl acetate and 0.75 $g$ butyl acetate. When another two hours have elapsed we add another dose of AIBN. After addition of the second injection of AIBN we dilute the reaction with 16.6 g ethyl acetate and 8.3 g butyl acetate. We let the reaction proceed for 15 hours. After cooling to room temperature, the stabiliser reaction mixture is used directly in the synthesis of the particles. The resulting product is highly viscous and has a golden colour.

## B. Synthesis of PMMA colloidal particles

For the synthesis of colloidal particles made out of poly(methyl methacrylate) (PMMA)[2] we add 49.0 g Methyl metacrylate (98% of total monomer weight), 1.0 g Methacrylic acid (2% of total monomer weight), 29.8 g Hexane, 14.3 g Mineral Oil, and approximately 10 mg of DiO-C18 fluorescent dye to a 250 mL round-bottom flask. We add a small magnetic stirring bar and stir the solution until all the dye has dissolved. We then add 5 g of PMMA-g-PHSA stabiliser, 390 mg AIBN, and 300 mg 1-Octanethiol. The reaction takes place under reflux conditions at 80 $^{\circ}C$ and proceeds for 2 hours under slow magnetic stirring. We then filter the reaction mix through glass wool. Reaction products are removed by cleaning the suspension through centrifugation against hexane (2x). The resulting particles have a radius of 710 nm as measured by static light scattering (Fig. S1A). By increasing the monomer amount in the reaction, the particle size can be increased. Using this method we synthesise a second batch of particles with a radius of 975 nm as determined by SLS (Fig. S1B).

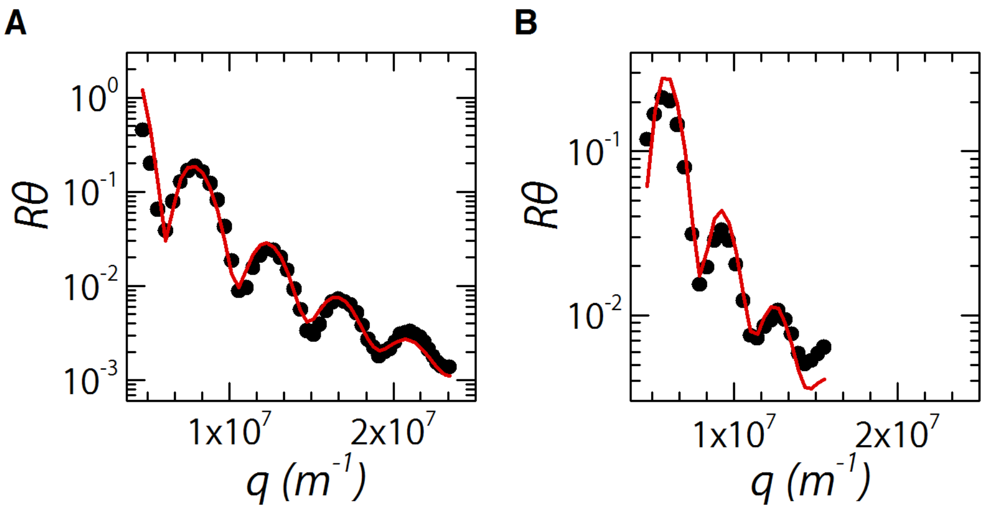


Figure S1. **Size determination of colloidal particles with SLS.** (**A**) Rayleigh ratio as a function of scattering vector for the smaller particles **q**, solid red line is a theoretical fit as calculated using Mie theory giving a radius of gyration of 710 nm (black circles). (**B**) Same as in (**A**) but for particles with a radius of gyration of 975 nm.

## II. SAMPLE PREPARATION

*Washing and density matching of particle suspension* - We start by washing, by sequential centrifugation and re-suspension steps, the particle suspensions two times with a 50/50 volume-% mix of *cis*-Decahydronaphthalene (cDec) and Tetrachloroethylene (TCE) with 10 mM AOT. By varying the relative volumes of cDec and TCE we can density match our particles with the solvent mix. We achieve this by adding small amounts of TCE or cDec until we can no longer observe sedimentation after centrifugation at 2000 g for one hour. The density matched suspension is also matched well enough in refractive index to allow us to examine the samples using confocal microscopy up to depths of approximately 150 $\mu m$, without loss of resolution due to scattering. After density matching the particle suspensions we concentrate the suspension by centrifuging at 2500 g and 35 $^{\circ}C$ until we observe a clear supernatant. We decant the supernatant and store it for use later. All subsequent samples are made from this concentrated stock suspension and are diluted with the supernatant, if necessary. *Sample chamber fabrication* - Our sample chambers are constructed by gluing, using Norland Optical Adhesive 61 UV curable glue, two 21 mm x 26 mm microscopy cover slips on a larger round cover slip (radius of 2.5 cm); leaving a space between them of approximately 0.5 cm. We than glue a microscope slide (26 mm x 76 mm) across the two rectangular cover slips using the same UV glue. This creates a hollow chamber with dimension of approximately 5 mm x 26 mm x 150 $\mu m$. We load the sample chambers using capillary forces and seal both ends of the chamber with 2-component gel epoxy from VersaChem.

## III. PAIR POTENTIAL U(R)

The pair potentials $U(r)$ is obtained from the measured radial distribution function $g(r)$ using the Ornstein-Zernike relation:

$$h(r) = c(r) + \rho \int h(r)c(r-r)d\mathbf{r} \tag{1}$$

where $h(r) = g(r) - 1$ is the total correlation function, $c(r)$ the direct correlation function, and $\rho$ the number density of particles. We solve this equation by Fourier transformation, using the hypernetted chain (HNC) closure approximation:

$$c(r) = k_B T U(r) + h(r) - lng(r) \tag{2}$$

This closure approximation is known to give accurate results for soft potentials at not too high densities[3].

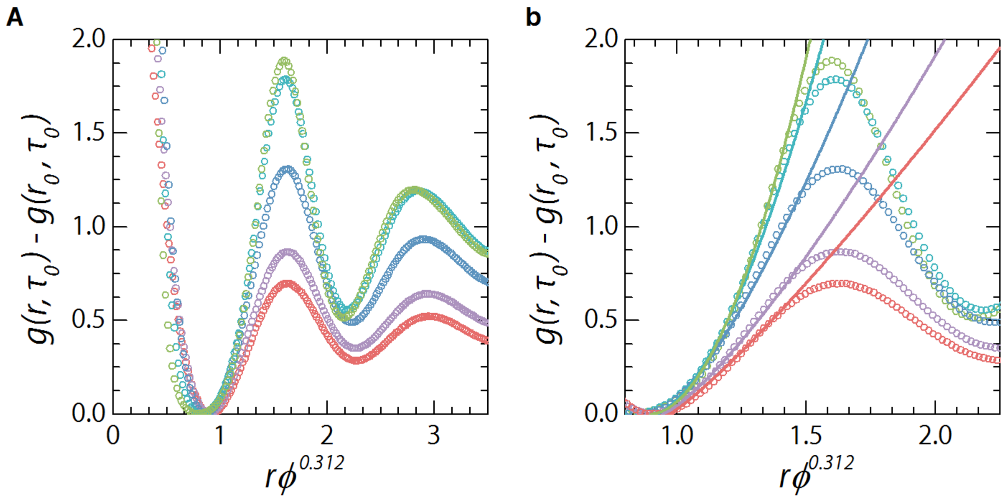


Figure S2. (**A**) The van Hove function for the different packing fractions $\phi$ in the rescaled coordinate system $u = r\phi^{0:312}$. (**B**) Power law fit to the left flank of the van Hove function $g(r, \tau_0)$.

## IV. SCALING OF $Z(\phi)$

### A. Power law fit to the the rescaled van Hove function

It is possible to capture the behaviour of the coordination number $Z(\phi, \tau_0)$ by mimicking the variation of the steepness of the left flank of the main peak of $g(r, \phi, \tau_0)$ with a simple power law. To this end, it will be useful to rescale the $r$-axis such that the position of the main peak for different $\phi$ align. This alignment is achieved by mapping the van Hove functions on the new coordination $u = r\phi^{0.312}$ (Fig. S2A).

Subsequently, the fitting of the ascending flank of the main peak can be carried out with a power law $g(u, \tau_0) = a(u - b)^c$. The result of this procedure is depicted in Figure S2B. The parameters $a$, $b$ and $c$ are $\phi$-dependent, and can be approximated by

$$\begin{aligned} a(\phi) =& 124.7\ \phi^{2.75} \\ b(\phi) =& 0.76\ \phi^{-0.139} \\ c(\phi) =& 5.54\ \phi^{0.95}. \end{aligned}$$

In order to simplify the approximation we assume that the slowly varying offset $b$ is constant for different $\phi$. We set it so its maximum value $b = 0.965$, which is attained for $\phi = 0.18$, thus, introducing a small error for larger $\phi$. Plugging the fitting functions $a$, $b$, and $c$ back into the expression for $g(r, \tau_0)$ yields the approximate form of the ascending flank of the van Hove correlation as

$$g(r, \phi, \tau_0) = 124.7\ \phi^{2.75}\ (u - 0.965)^{5.54\ \phi^{0.95}}$$

where $u = r\phi^{0.312}$. The coordination number $Z(\phi, \tau_0)$ can then be approximately computed as

$$\begin{aligned} Z(\phi, \tau_0) =& 4\phi \frac{\phi}{\frac{4\pi}{3} a^3} \phi^{-0.936} \int_{0.965}^{1.616} u^2 g(u, \phi, \tau_0)\, \mathrm{d}u \\ =& \frac{420.584\, \phi^{2.814} e^{-181.163\phi^{0.95}}}{2.790\phi^{2.85} + \phi^{0.95} + 3.022\phi^{1.9} + 0.0985} \\ & \cdot \Big( e^{2.382\phi^{0.95}} \left(-6.272 \cdot 10^{-15}\phi^{0.95} - 6.95 \cdot 10^{-15}\phi^{1.9} - 1.359 \cdot 10^{-15}\right) \\ & + e^{178.781\phi^{0.95}} \left(\phi^{0.95} + 1.321\phi^{1.9} + 0.168\right)\Big)\,. \end{aligned} \tag{3}$$

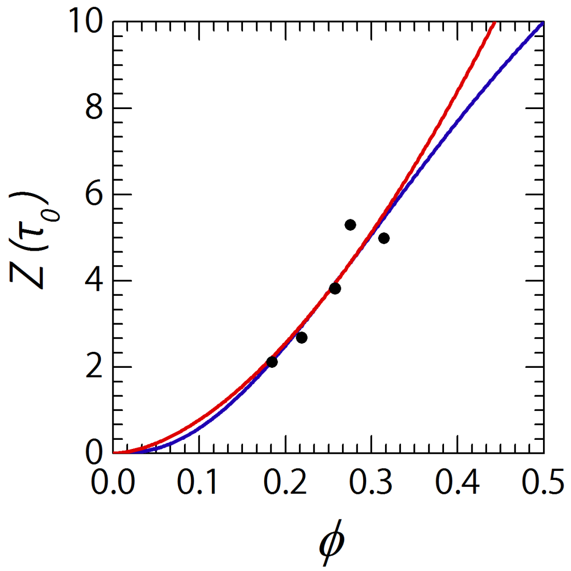


Figure S3. Plot showing the data points evaluated directly from the experimental van Hove function compared to the behaviour of $Z(\phi)$ obtained from the approximation (blue curve) and the power law fit (orange curve).

It should be noted that inherently this approximation should become less accurate towards higher $\phi$ since in clearly overestimates the height of the main peak, as can be seen from Figure S2B. The plot of expression (3) is shown in Figure S3. We observe that in the experimentally probed range of $\phi$ the simple power law for $Z(\phi)$ represents a reasonable approximation to the expression (3) directly obtained from the change of slope of the van Hove function.


[1] M. T. Elsesser and A. D. Hollingsworth, Langmuir **26**, 17989 (2010).

[2] L. Antl, J. W. Goodwin, R. D. Hill, R. H. Ottewill, S. M. Owens, S. Papworth, and J. A. Waters, Colloids and Surfaces **17**, 67 (1986).

[3] S. H. Behrens and D. G. Grier, Physical Review E **64**, 050401 (2001).

## V. SUPPLEMENTAL FIGURES AND MOVIES

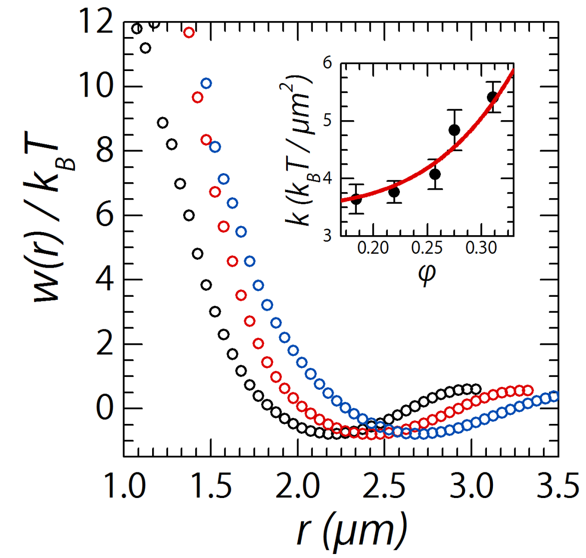


Figure S4. The potentials of mean force calculated as the negative natural logarithm of the $g(r)$ for $\phi = 0.31$, 0.26, and 0.18. *inset* Effective bond spring constant determined by fitting the minimum of $w(r)$ to a harmonic well, for $\phi = 0.31$, 0.28, 0.26, 0.22, and 0.18. The solid line is a power law fit to the data.

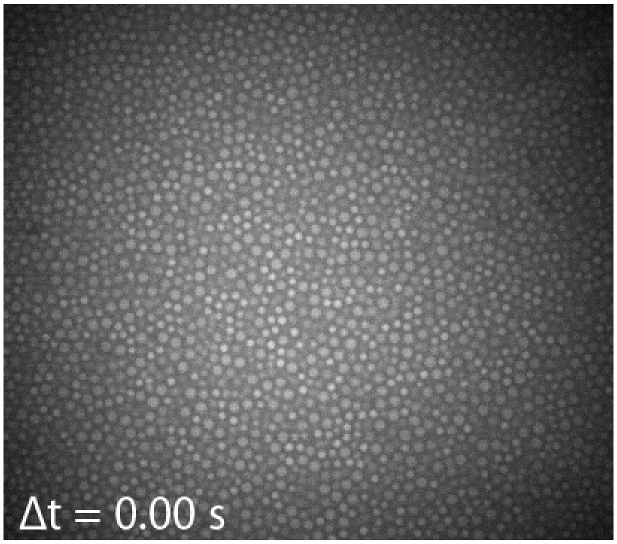


Figure S5. **Raw confocal data - High volume fraction.** Raw experimental data for $\phi = 0.35$ with a real time duration of 10 s. Shown here is a still from the movie. Available at `https://youtu.be/nfHl9gsU3lI`

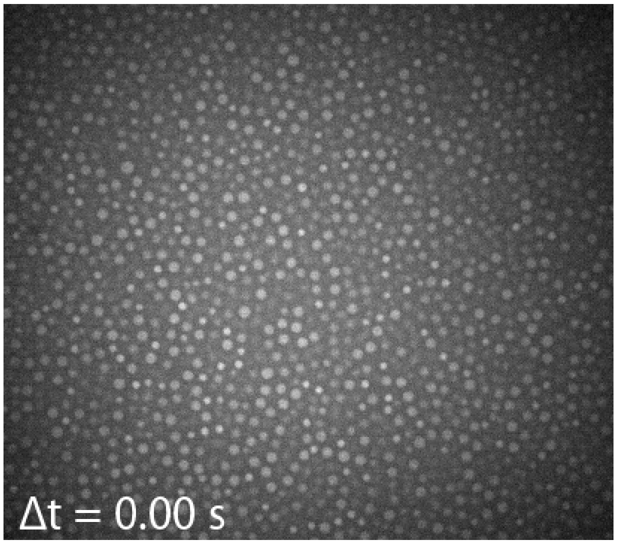


Figure S6. **Raw confocal data - Low volume fraction.** Raw experimental data for $\phi = 0.18$ with a real time duration of 10 s. Shown here is a still from the movie. Available at `https://youtu.be/5396_8LRpeQ`

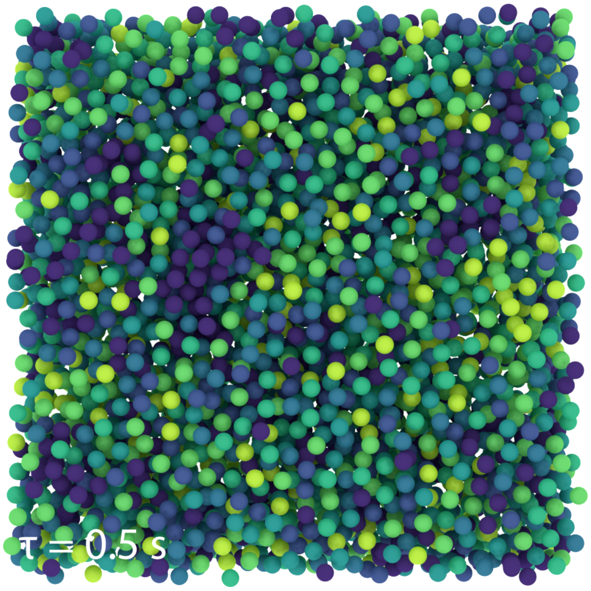


Figure S7. **Decay of $Z$ with increasing lag time.** We show the decay of the long-lived bond network with increasing delay $\tau$. Particles are coloured according to $Z$ at constant experimental time $t$ and varying delay $\tau$ from 0.5 s to 171 s, as shown in the video. Shown here is a still from the movie. Available at `https://youtu.be/_g20Ic4eKsY`

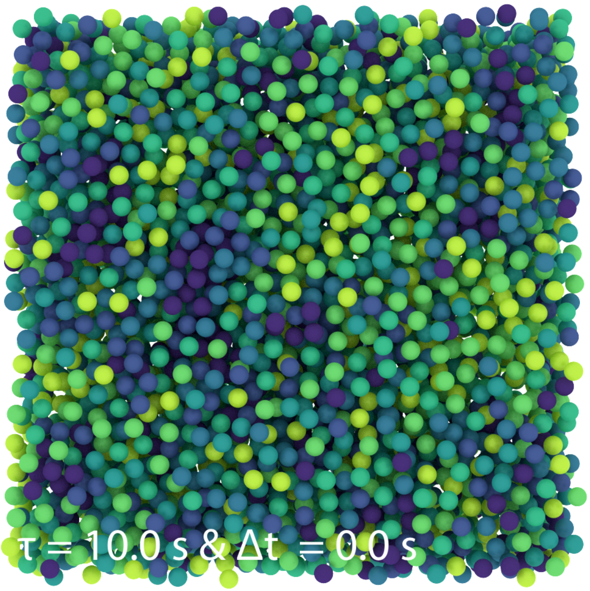


Figure S8. **Dynamics of $Z$ clusters.** Here we show the dynamical behaviour of $Z$ at a constant delay time $\tau = \tau_0$ while varying the experimental time as indicated in the video. Shown here is a still from the movie. Available at `https://youtu.be/q5N0gfNTfME`
